# Supplementary material for: ORRB -- OpenAI Remote Rendering Backend
Source: arXiv:1906.11633 source file (2019-06-26)
Supplement: Supplementary file 1 [file background.tex]

\section{Reinforcement Learning Background}\label{sec:rl}

% BB: I think we can drastically cut down on the RL background if we want to cut. We could potentially merge PPO and GAE into 1 shorter section. We could also merge and shorten DDPG into SAC because we don't actually use base DDPG anymore. UVFA and HER could be shortened into 1 or 2 sentences each.}

\subsection{Reinforcement Learning (RL)}

We consider the standard reinforcement learning formalism
consisting of an agent interacting with an environment.
To simplify the exposition we assume in this section that the environment is fully observable.\footnote{The environments
we consider in the paper are only partially observable.}
An environment
is described by
a set of states $\S$,
a set of actions $\A$,
a distribution of initial states $p(s_0)$,
a reward function $r : \S \times \A \rightarrow \R$,
transition probabilities $p(s_{t+1}|s_t,a_t)$,
and a discount factor $\gamma \in [0,1]$.

A policy $\pi$ is a mapping from state to a distribution over actions.
Every episode starts by sampling an initial state $s_0$.
At every timestep $t$ the agent produces an action based on the current state:
$a_t \sim \pi(\cdot|s_t)$.
In turn, the agents receives a reward $r_t=r(s_t,a_t)$ and the environment's new state $s_{t+1}$, which is sampled from the distribution $p(\cdot|s_t,a_t)$.
The discounted sum of future rewards, also referred to as the \emph{return}, is defined as
$R_t=\sum_{i=t}^\infty \gamma^{i-t} r_i$.
The agent's goal is to maximize its expected return $\E [R_0|s_0]$, where
the expectation is taken over the initial state distribution, policy, and environment transitions accordingly to the dynamics
specified above.
The \emph{Q-function} or \emph{action-value} function is defined as $Q^\pi(s_t,a_t)=\E[R_t|s_t,a_t]$, while the
\emph{V-function} or \emph{state-value} function is defined as $V^\pi(s_t)=\E[R_t|s_t]$.
The value $A^\pi(s_t,a_t)=Q^\pi(s_t,a_t)-V^\pi(s_t)$ is called
the \emph{advantage} and tells whether the action $a_t$ is better or worse than an average
action the policy $\pi$ takes in the state~$s_t$.

%It is easy to show that the action-value function satisfies the following equation called
%the Bellman equation:
%$$Q^\pi(s,a) = \E_{s' \sim p(\cdot|s,a)} \left[ r(s,a) + \gamma Q^\pi(s', \pi(s')) \right].$$

%Let $\pi^*$ denote an \emph{optimal policy} i.e. any policy $\pi^*$ s.t. %$Q^{\pi^*}(s,a) \ge Q^\pi(s,a)$
%for every $s \in S, a \in A$ and any policy $\pi$.
%All optimal policies have the same Q-function which is called \emph{optimal %Q-function} and denoted $Q^*$.
%It is easy to show that it satisfies the following equation called
%the \emph{Bellman} equation:
%$$Q^*(s,a) = \E_{s' \sim p(\cdot|s,a)} \left[ r(s,a) + \gamma \max_{a' \in \A} %Q^*(s', a') \right].$$

\subsection{Generalized Advantage Estimator (GAE)} \label{sec:gae}

Let $V$ be an approximator to the value function of some policy, i.e. $V \approx V^\pi$.
The value $$\hat{V}_t^{(k)}=\sum_{i=t}^{t+k-1} \gamma^{i-t} r_i + \gamma^{k} V(s_{t+k}) \approx V^\pi(s_t,a_t)$$
is called the $k$-step return estimator.
The parameter $k$ controls the bias-variance tradeoff of the estimator
with bigger values resulting in an estimator closer
to empirical returns and having less bias and more variance.
\emph{Generalized Advantage Estimator (GAE)} \citep{gae}
is a method of combining multi-step returns in the following way:
$$\hat{V}_t^\text{GAE} = (1-\lambda) \sum_{k>0}\lambda^{k-1} \hat{V}_t^{(k)} \approx V^\pi(s_t,a_t),$$
where $0<\lambda<1$ is a hyperparameter. Using these to estimate the \emph{advantage}:
$$\hat{A}_t^\text{GAE} = \hat{V}_t^\text{GAE} - V(s_t) \approx A^\pi(s_t,a_t).$$
It is possible
to compute the values of this estimator for all states
encountered in an episode in linear time \citep{gae}.

\subsection{Proximal Policy Optimization (PPO)} \label{sec:ppo}

\emph{Proximal Policy Optimization (PPO)} \citep{ppo} is one of the most popular on-policy RL algorithms.
It simultaneously optimizes a stochastic policy as well as an approximator to the value function.
%It optimizes a stochastic policy which given a state outputs a probability distribution from some class of probability distributions.
%In practice, a multivariate Gaussian distribution with diagonal covariance matrix is usually employed, and the policy outputs
%the mean and standard deviation of the action to be applied given the current observation.
PPO interleaves the collection of new episodes with policy optimization.
After a batch of new transitions is collected, optimization is performed
with minibatch stochastic gradient descent to maximize the objective $$L_{\text{PPO}}=\E \min \left( \frac{\pi(a_t|s_t)}{\pi_{\text{old}}(a_t|s_t)} \hat{A}^\text{GAE}_t,\, \mbox{clip}\left(\frac{\pi(a_t|s_t)}{\pi_{\text{old}}(a_t|s_t)},\,1-\epsilon,\,1+\epsilon \right)\hat{A}^\text{GAE} _t\right),$$ where
$\frac{\pi(a_t|s_t)}{\pi_{\text{old}}(a_t|s_t)}$ is the ratio of the probability of taking the given action under the current policy $\pi$ to the probability
of taking the same action under the old behavioral policy that was used to generate the data,
%$A$ is the estimate of the advantage function (usually GAE, See %Sec.~\ref{sec:gae}),
and $\epsilon$ is a hyperparameter (usually $\epsilon \approx 0.2$).
This loss encourages the policy to take actions which are better than average (have positive advantage)
while clipping discourages bigger changes to the policy by limiting how much can be gained
by changing the policy on a particular data point.
The value function approximator is trained with supervised learning with the target for $V(s_t)$ being $\hat{V}_t^\text{GAE}$.
To boost exploration, it is a common practice to encourage the policy to have high entropy of actions by including an entropy bonus in the optimization objective.
