# Supplementary material for: ORRB -- OpenAI Remote Rendering Backend
Source: arXiv:1906.11633 source file (2019-06-26)
Supplement: Supplementary file 2 [file calibration.tex]

\subsection{MuJoCo Model Calibration}
\label{app:model-calibration}

The MuJoCo XML model of the hand requires many parameters, which are then used as the mean of the randomized distribution of each parameter for the environment. Even though substantial randomization is required to achieve good performance on the physical robot, we have found that it is important for the mean of the randomized distributions to correspond to reasonable physical values. We calibrate these values by recording a trajectory on the robot, then optimizing the default value of the parameters to minimize error between the simulated and real trajectory.

To create the trajectory, we run two policies in sequence against each finger. The first policy measures behavior of the joints near their limits by extending the joints of each finger completely inward and then completely outward until they stop moving. The second policy measures the dynamic response of the finger by moving the joints of each finger inward and then outward in a series of oscillations. The recorded trajectory across all fingers lasts a few minutes.

To optimize the model parameters, these trajectories are then replayed as open-loop action sequences in the simulator. 
The optimization objective is to match joint angles after $1$ second of running actions. Parameters 
are adjusted using iterative coordinate descent until the error is minimized. We exclude modifications to the XML
that does not yield improvement over $0.1\%$.

For each joint, we optimize the damping, equilibrium position, static friction loss, stiffness, margin, and the minimum and maximum of the joint range. For each actuator, we optimize the proportional gain, the force range, and the magnitude of backlash in each direction.  Collectively, this corresponds to 264 parameter values.

%For each tendon, we optimize the damping, static friction loss, stiffness, and the minimum and maximum of the tendon range.
% woj: our tendons are fictitious. They are used to simulated unactuated joints. This text might indicate that we have actuat 
% tendons. Skipping it.
