# Supplementary material for: ORRB -- OpenAI Remote Rendering Backend
Source: arXiv:1906.11633 source file (2019-06-26)
Supplement: Supplementary file 3 [file episodic.tex]

\subsection{Truncated Episodic Replay Buffer}\label{app:episodic}

When using recurrent policies with experience replay, handling the hidden state correctly can be tricky.
While recurrent policies and value functions have been used in the past, they typically use backpropagation through time (BPTT) for the entire episode without truncation~\citep{rdpg, rpg, rpg2, recurrent-robot, peng2017sim} or use truncation but zero out initial hidden states~\citep{rdqn}.

In our setting, we can not replay entire episodes because the are very long and have vastly varying lengths,
which would render large batch optimization impossible.
An alternative is to split each episode into chunks,
record the hidden state at the beginning of each chunk at the time of episode
generation, and use it when replaying the chunk.
Surprisingly, we noticed using even slightly stale
hidden state (a few minutes old) results in inferior performance compared to
replaying starting from a correct hidden state.

To address this issue, we update the hidden states stored in the replay buffer during optimization.
More precisely, 
after processing a chunk, we update the network and also update the initial hidden state of the \emph{next} chunk using the final hidden state of the \emph{current} chunk and process episodes chunk by chunk in order.
