# Supplementary material for: ORRB -- OpenAI Remote Rendering Backend
Source: arXiv:1906.11633 source file (2019-06-26)
Supplement: Supplementary file 4 [file hardware-full.tex]

\section{Hardware Description}
\label{app:hardware}

% \todo{maybe use this figure or parts of it?}
% \begin{figure}\centering
%     \includegraphics[width=\textwidth]{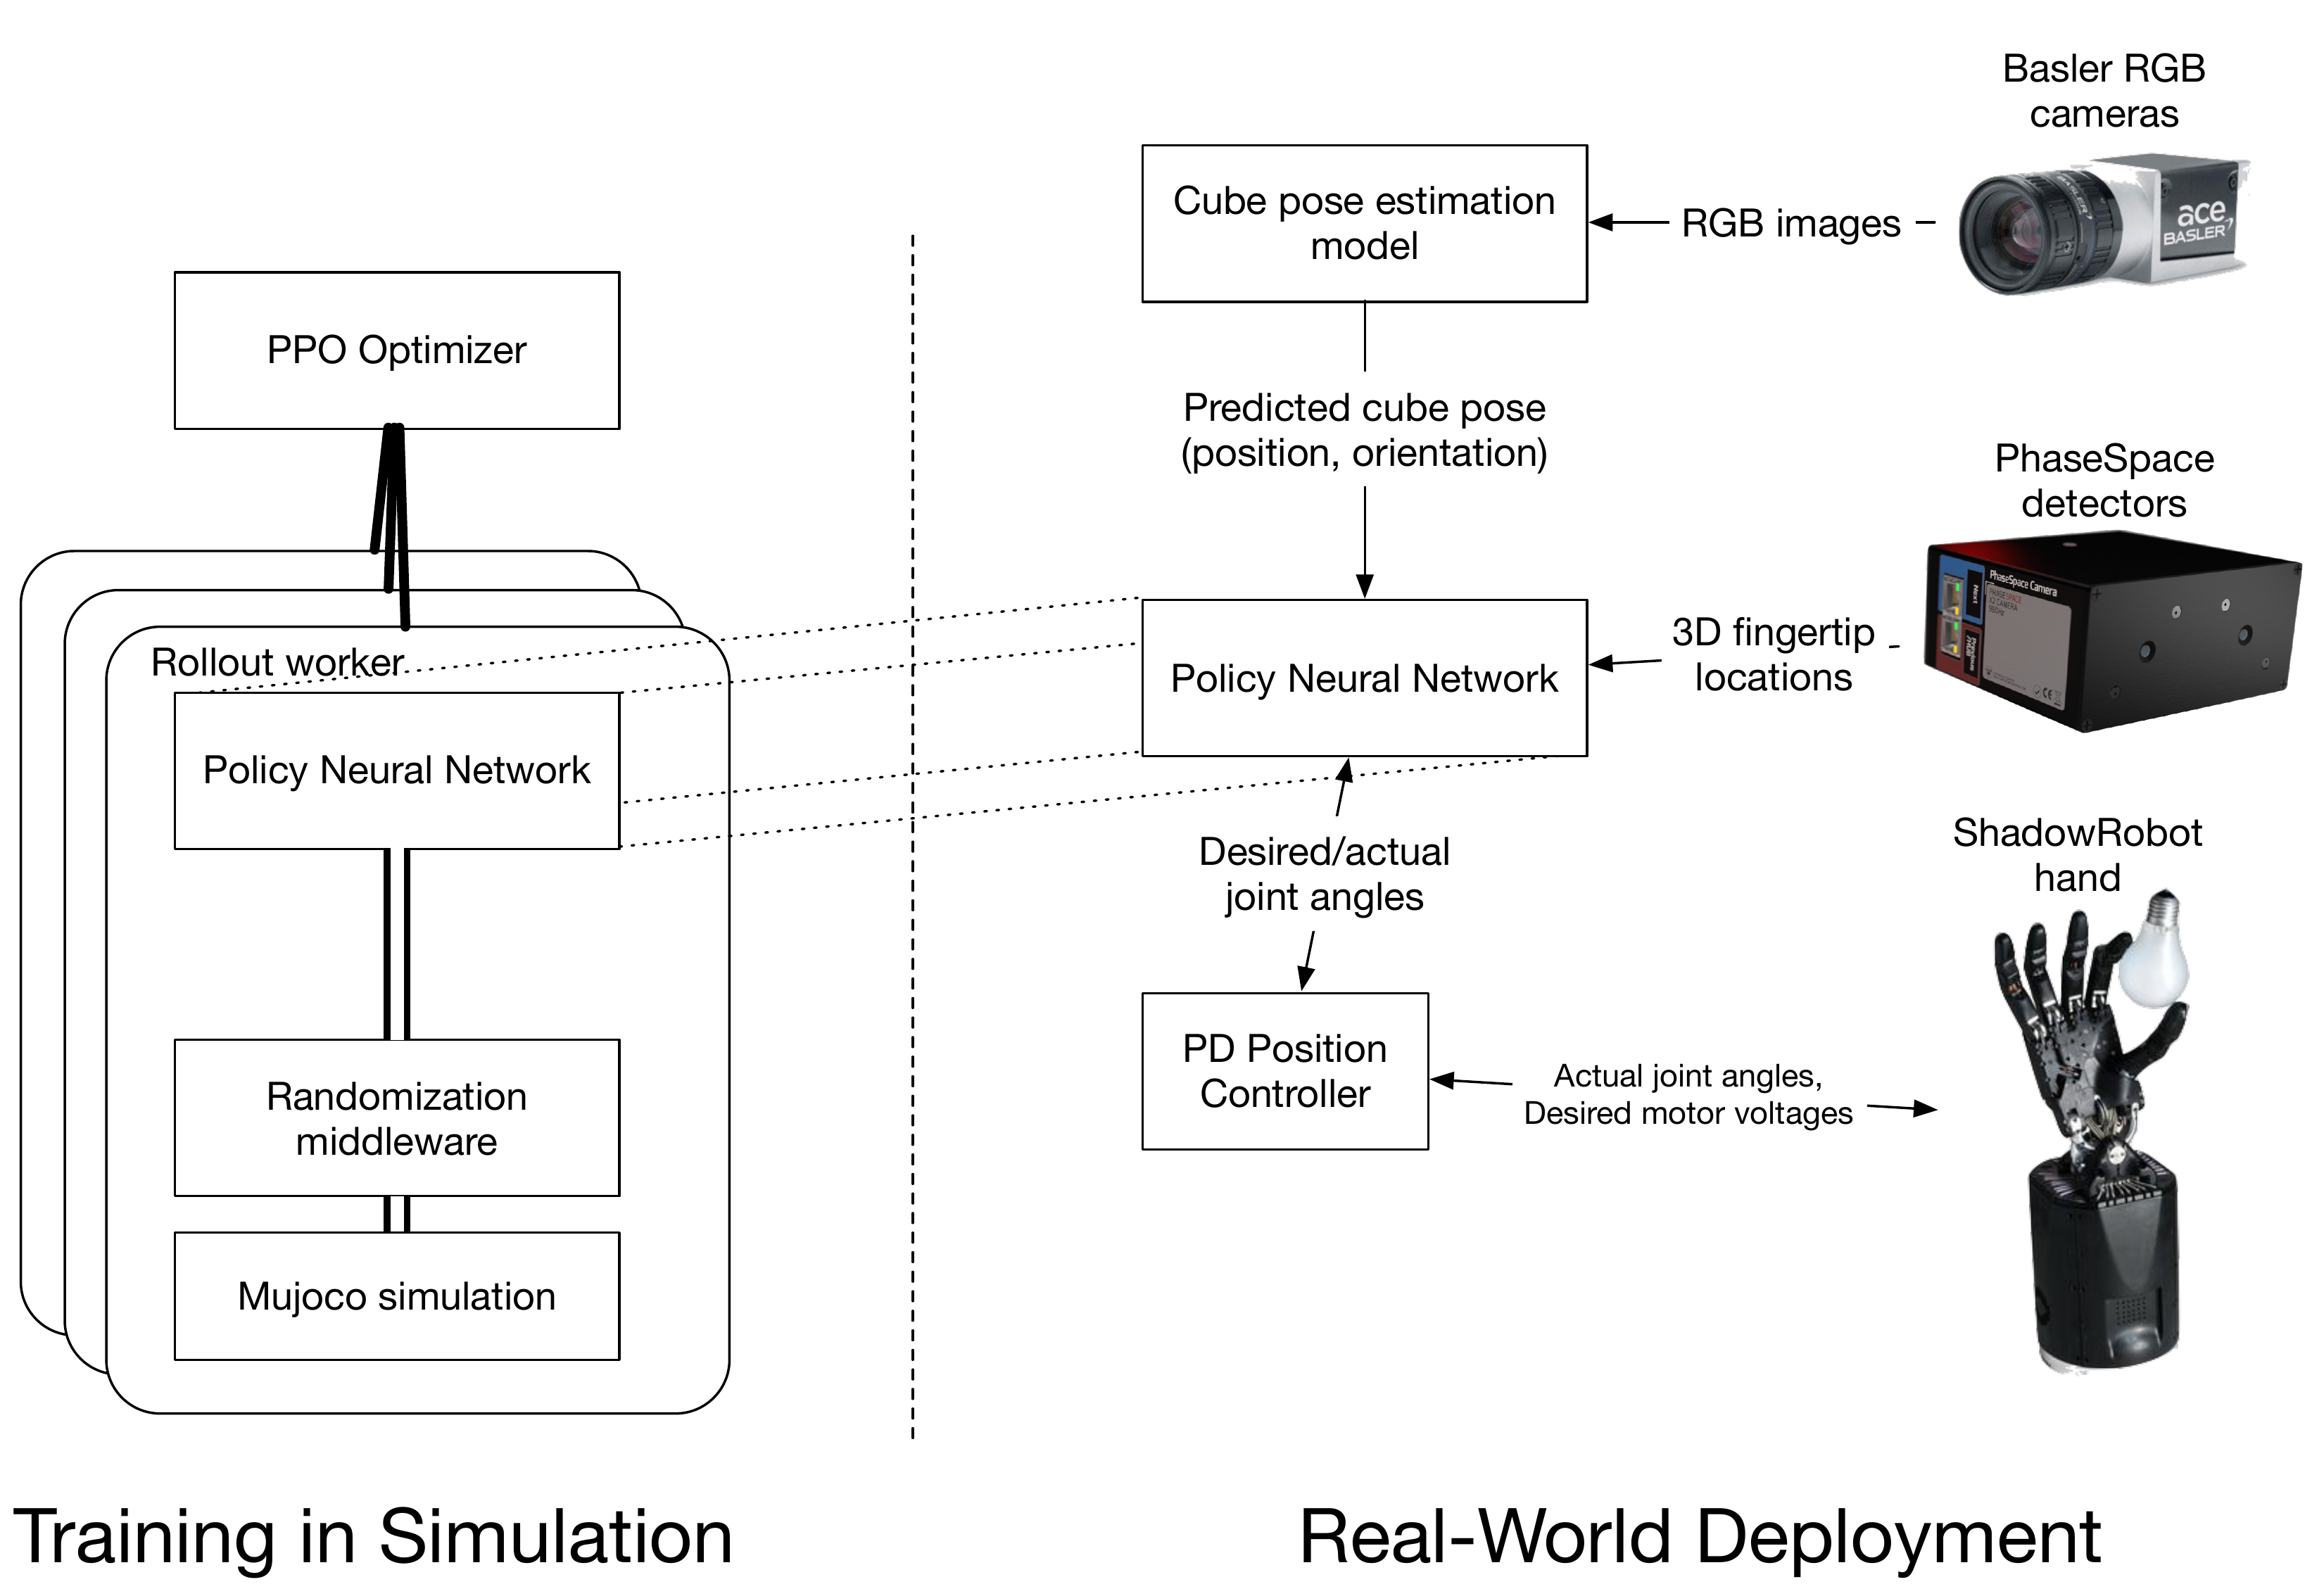}
% \end{figure}

\subsection{ShadowRobot Dexterous Hand}

We use the ShadowRobot Dexterous Hand. Concretely, we use the version with electric motor actuators, EDC hand (EtherCAT-Dual-CAN).

The hand has \num{24} degrees of freedom between its links and is actuated by \num{40} Spectra tendons controlled by \num{20} DC motors in the base of the hand, each actuating a pair of agonist--antagonist tendons connected via a spool.
\num{16} degrees of freedom can be controlled independently whereas the remaining \num{8} joints (which are the joints between the non-thumb finger proximal, middle, and distal segments) form $4$ pairs of coupled joints.

\subsection{PhaseSpace Visual Tracking}
We use a 3D tracking system to localize the tips of the fingers, to perform calibration procedures, and as ground truth for the RGB image-based tracking. The PhaseSpace Impulse X2E tracking system uses active LED markers that blink to transmit a unique ID code and linear detector arrays in the cameras to detect the positions and IDs. The system features capture speeds of up to 960 Hz and positional accuracies of below 20 $\mu$m. The data is exposed as a 3D point cloud together with labels associating the points with stable numerical IDs. Our setup uses 16 cameras distributed spherically around the hand and centered on the palm with a radius of approximiately $0.8$ meters.

\subsection{RGB Cameras} \label{app:cameras}
We also use RGB images to track the objects for manipulation. We perform object pose estimation using 3 Basler acA640-750uc RGB cameras with a resolution of 640x480 placed approximately 50 cm from the Shadow hand. We use 3 cameras to resolve pose ambiguities that may occur with monocular vision. We chose these cameras for their flexible parameterization and low latency. Figure \ref{fig:camera-setup} shows the placement of the cameras relative to the hand.

\begin{figure}[t]
    \centering
    \includegraphics[width=0.9\textwidth]{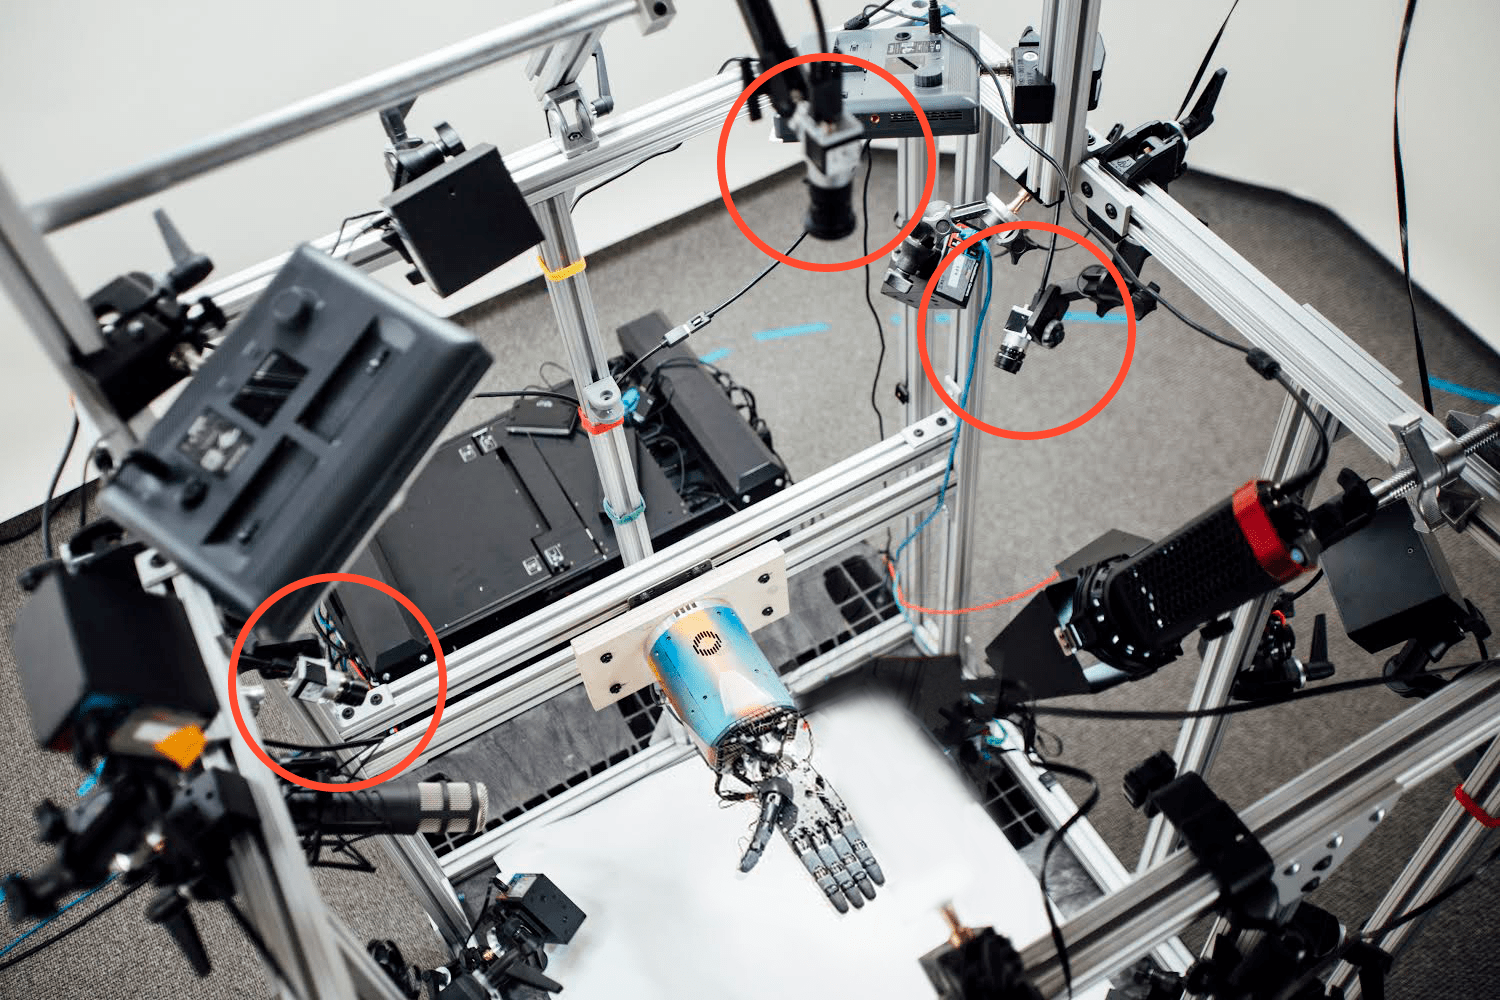}
    \caption{Our 3-camera setup for vision-based state estimation.}
    \label{fig:camera-setup}
\end{figure}

\subsection{Control}

The high-level controller is implemented as a Python program
running a neural network policy implemented in Tensorflow~\citep{tensorflow}
on a GPU. Every 80ms it queries the Phasespace sensors and then runs inference with the neural network to obtain the action, which takes roughly 25ms. The policy outputs an action that specifies the change of position for each actuator, relative to the current position of the joints controlled by the actuator. It then sends the action to the low-level controller.

The low-level controller is implemented in C++ as a separate process on a different machine which is 
connected to the Shadow hand via an Ethernet cable. The controller is written as a real-time system 
--- it is pinned to a CPU core, has preallocated memory, and does not depend on any garbage collector to avoid non-deterministic delays.
The controller receives the relative action, converts it to 
an absolute joint angle and clips to the valid range, then sets each component of the action as the target for a PD controller. Every 5ms, the PD controller queries the Shadow hand joint angle sensors, then attempts to achieve the desired position.

Surprisingly, decreasing time between actions to 40ms increased training time but did not noticeably improve performance in the real world.

\subsection{Joint Sensor Calibration} 
\label{app:sensor-calibration}
The hand contains 26 Hall effect sensors that sense magnetic field rotations along the joint axis.
%Some joints contain more than one sensor.
%We use the calibration procedure described below to transform these into measurements of the joint angles. \todo{move somewhere else}
To transform the raw magnetic measurements from the Hall sensors into joint angles, we use a piecewise linear function interpolated from 3-5 truth points per joint. To calibrate this function, we initialize to the factory default created using physical calibration jigs. For further accuracy, we attach PhaseSpace markers to the fingertips, and minimize error between the position reported by the PhaseSpace markers and the position estimated from the joint angles.
We estimate these linear functions by minimizing reprojection error with \texttt{scipy.minimize}.
