# Supplementary material for: ORRB -- OpenAI Remote Rendering Backend
Source: arXiv:1906.11633 source file (2019-06-26)
Supplement: Supplementary file 5 [file hyperparameters.tex]

\FloatBarrier
\section{Optimization Details}\label{app:hyper}
\subsection{Control Policy}\label{app:hyper-ppo}

%\subsection{PPO Hyperparameters}\label{app:ppo-hyper}
We normalize all observations given to the policy and value networks with running means and standard deviations. We then clip observations such that they are within 5 standard deviations of the mean. We normalize the advantage estimates within each minibatch. We also normalize targets for the value function with running statistics. The network architecture is depicted in \autoref{fig:ppo}.

\begin{figure}[t]
    \begin{minipage}[c]{0.6\textwidth}
        \includegraphics[width=0.9\textwidth]{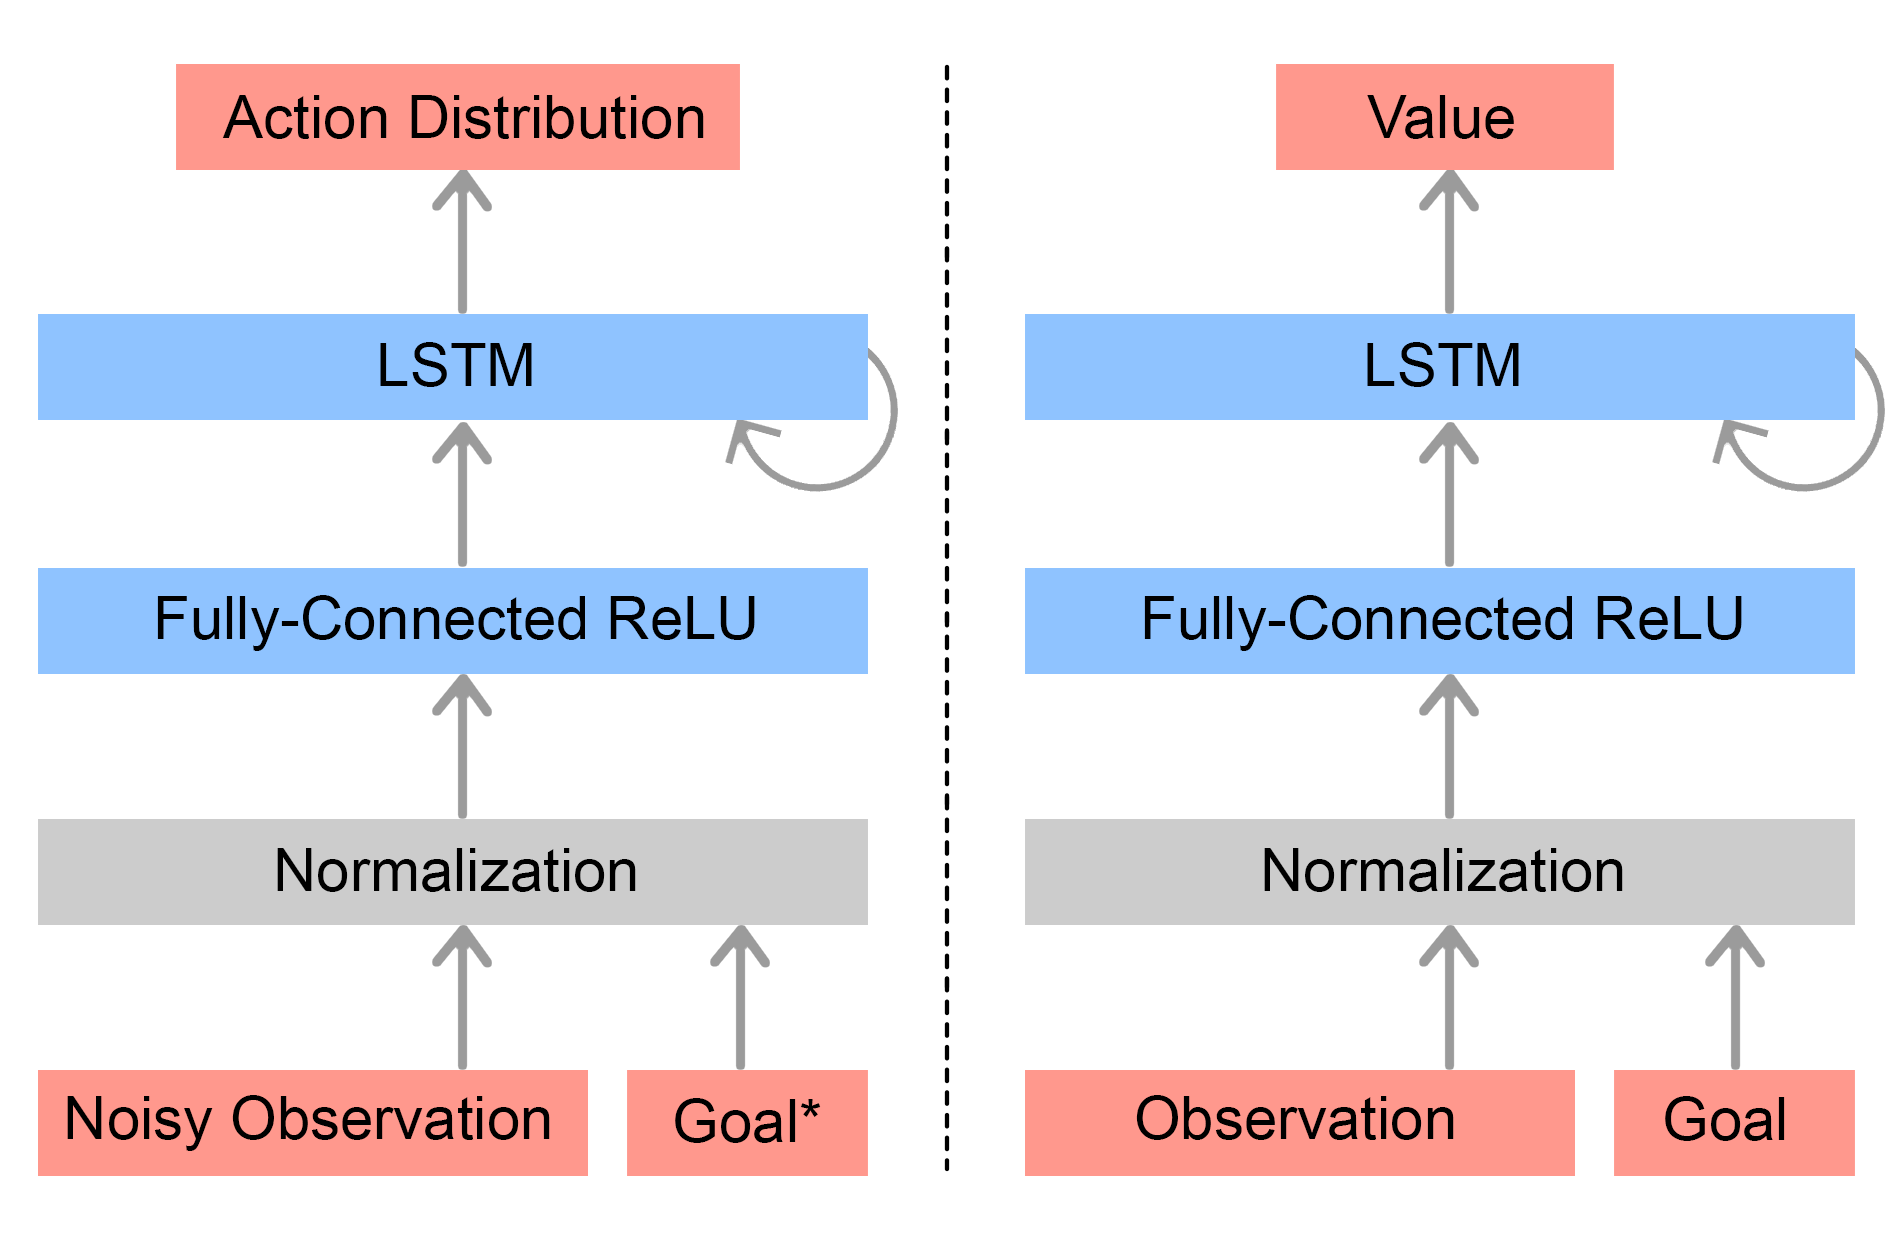}
    \end{minipage}\hfill
    \begin{minipage}[c]{0.4\textwidth}
        \caption{Policy network (left) and value network (right). Each network consists
        of an input normalization, a single fully-connected hidden layer with ReLU activations \citep{relu}
        and a recurrent LSTM block \citep{lstm}. The normalization block
        subtracts the mean value of each coordinate (across all data gathered so far),
        divides by the standard deviation, and removes outliers by clipping.
        There is no weight sharing between the two networks.
        The goal provided to the policy is the noisy relative target orientation (see \autoref{table:policy-inputs} for details).}
        \label{fig:ppo}
    \end{minipage}
\end{figure}

\begin{table}[h!]
    \footnotesize
    \centering
    \caption{Hyperparameters used for PPO.}
    
    \begin{tabular}{@{}ll@{}}
        \toprule
        \textbf{Hyperparameter} & \textbf{Value} \\ \midrule
        hardware configuration & 8 NVIDIA V100 GPUs + 6144 CPU cores \\ 
        action distribution & categorical with $11$ bins for each action coordinate \\
        discount factor $\gamma$ & $0.998$ \\
        Generalized Advantage Estimation $\lambda$ & $0.95$ \\
        entropy regularization coefficient & $0.01$ \\
        PPO clipping parameter $\epsilon$ & $0.2$ \\
        optimizer & Adam~\citep{adam} \\
        learning rate & 3e-4 \\
        %MA: Commenting because it's difficult to understand
        %max normalized gradient norm\footnotemark & 5.0 \\
        batch size (per GPU) & $80$k chunks x $10$ transitions = $800$k transitions \\
        minibatch size (per GPU) & $25.6$k transitions \\
        number of minibatches per step & $60$ \\
        network architecture & dense layer with ReLU + LSTM \\
        size of dense hidden layer & 1024 \\
        LSTM size & 512 \\
    \bottomrule\end{tabular}
    \label{tbl:ppo}
\end{table}
%\footnotetext{We clip gradients so they are within 5.0 std dev's of mean}

\FloatBarrier

%\section{Vision to State Training Hyperparameters}

%Details for vision to state estimator hyperparameters are given in \autoref{tbl:vision-hyp}.

% \todo{Alex/Mac: add missing details}
\subsection{Vision Model}\label{app:vision-hyper}\label{app:vision_training}
Vision training hyperparameters are given in \autoref{tbl:vision-hyp} and the details of the model architecture are given in \autoref{tbl:vision-hyper-arch}.

We also apply data augmentation for training. More specifically, we leave the object pose as is with $20\%$ probability, rotate the object by $90^{\circ}$ around its main axes with $40\%$ probability, and ``jitter'' the object by adding Gaussian noise to both the position and rotation indepdently with $40\%$ probability.

% MA: removed because we already say in the paper that the parameters are shared
%The layers labeled "Each" are shared image towers that are individually run over each input image.
%The outputs of the individual image towers are concatenated and the final output is generated from that result.
%For all Conv2D, ResNet, and Fully Connected Layers (except the final output layer) use ReLU activations.

\begin{table}[h!]
    \centering
    \footnotesize
    \caption{Hyperparameters used for the vision model training.}
    
    \begin{tabular}{@{}ll@{}}
        \toprule
        \textbf{Hyperparameter} & \textbf{Value} \\ \midrule
        hardware configuration & 3 NVIDIA P40 GPUs\footnote{Two GPUs are used for rendering and one for the optimization.} + 32 CPU cores  \\
        optimizer & Adam~\citep{adam} \\
        learning rate & $0.0005$, halved every $20\,000$ batches \\
        minibatch size &  $64 \times 3 = 192$ RGB images \\
        image size & $200 \times 200$ pixels \\
        weight decay regularization & $0.001$ \\
        number of training batches & $400\,000$ \\
        network architecture & shown in \autoref{fig:vision-architecture} \\
    \bottomrule\end{tabular}
    \label{tbl:vision-hyp}
\end{table}
%\footnotetext{Since we have three cameras, this means that we actually use $64 \times 3 = 192$ RGB images per minibatch.}

        % camera_network = [['C', 5, 1, 32],
        %                   ['C', 3, 1, 32],
        %                   ['P', 3, 3],
        %                   ['R', 'building_block', 1, 3, 16],
        %                   ['R', 'building_block', 2, 3, 32],
        %                   ['R', 'building_block', 2, 3, 64],
        %                   ['R', 'building_block', 2, 3, 64],
        %                   ['SSM'],
        %                   ['FLAT']]

        % shared_network = [['FC', 128]]

\begin{table}[h!]
    \centering
    \footnotesize
    \caption{Hyperparameters for the vision model architecture.}
    \begin{tabular}{@{}ll@{}}
        \toprule
        \textbf{Layer} & \textbf{Details} \\ \midrule
        Input RGB Image & $200\times200\times3$ \\
        Conv2D & 32 filters, $5\times5$, stride 1, no padding \\
        Conv2D & 32 filters, $3\times3$, stride 1, no padding \\
        Max Pooling & $3\times3$, stride 3 \\
        ResNet & 1 block, 16 filters,  $3\times3$, stride 3 \\
        ResNet & 2 blocks, 32 filters, $3\times3$, stride 3 \\
        ResNet & 2 blocks, 64 filters, $3\times3$, stride 3 \\
        ResNet & 2 blocks, 64 filters, $3\times3$, stride 3 \\
        Spatial Softmax & \\
        Flatten & \\
        Concatenate & all 3 image towers combined\\ \midrule
        Fully Connected & 128 units \\
        Fully Connected & output dimension ($3$ position + $4$ rotation) \\
    \bottomrule\end{tabular}
    \label{tbl:vision-hyper-arch}
\end{table}

% \todo{Alex: architecture details}

 \FloatBarrier
