# Supplementary material for: ORRB -- OpenAI Remote Rendering Backend
Source: arXiv:1906.11633 source file (2019-06-26)
Supplement: Supplementary file 6 [file policy_obs.tex]

\section{Policy Observations}
\label{app:policy_obs}

As illustrated in the network architecture in~\autoref{fig:ppo}, we train two neural networks
--- a policy network and a value function network.
Because the policy network is expected to process inaccurate readings from the real world tracking sensors, we feed noisy observations into the network.
The original observations and several features that can only be tracked in the simulator are inputs to the value network to facilitate the model training. We don't need to collect those features from the robot, as the value network is not used during the physical deployment.

The complete lists of input features to both networks are described in~\autoref{table:policy-inputs}. The absolute goal is the desired object orientation. The relative goal is the difference between the current object orientation and the desired one.

\begin{table}[h!]
    \footnotesize
    \centering
    \caption{The inputs to the policy and value networks.}
    
    \begin{tabular}{@{}lll@{}}
        \toprule
        \textbf{Input type} & \textbf{Policy network} & \textbf{Value network} \\
        \midrule
        Goal & Noisy relative goal & Relative goal \\
        & -                   & Absolute goal \\
        \hline
        PhaseSpace & Noisy fingertip positions & Fingertip positions \\
                   & Noisy object position & Object position \\
                   & -                     & Object orientation in quaternions \\
        \hline
        Mujoco simulator-only & - & Hand joint angles \\
                              & - & Hand joint velocities \\
                              & - & Object velocity () \\
        %\hline
        % I remove this because there is no way it makes any difference
        % Termination criteria & Whether the object has fell off the hand &  Whether the object has fell off the hand \\
        \bottomrule
    \end{tabular}
\label{table:policy-inputs}
\end{table}
