# Supplementary material for: ORRB -- OpenAI Remote Rendering Backend
Source: arXiv:1906.11633 source file (2019-06-26)
Supplement: Supplementary file 7 [file randomizations.tex]

\subsection{Randomizations}
\label{app:randomizations}

A variety of randomizations are applied to the simulator, shrinking the reality gap between the simulated environment and the physical world in order to learn a policy that generalizes to reality.

\paragraph{Physical parameters.}
The physical parameters are sampled at the beginning of every episode and held fixed for the whole episode. The full set of randomized values are displayed in~\autoref{table:rand-physics}.

\paragraph{Observation noise.}
%
% On the physical robot, we installed $3$ motion capture markers on the hand base and one marker per fingertip so that the PhaseSpace system can figure out the hand position and track fingertip positions. The object position and orientation are tracked by PhaseSpace as well. All the readings on the physical system are noisy, and therefore we add noise
% to the exact observations computed in the simulator. In particular
We use two types of noise ---
\textit{correlated} noise which is sampled once per episode and kept fixed,
and an \textit{uncorrelated} Gaussian one.
Apart from Gaussian correlated noise, we also add more structured noise
coming from inaccurate placement of the motion capture markers
by computing the observations using slightly misplaced
markers in the simulator.
The configuration of noise levels is described in~\autoref{table:obs-noise}.
The observation noise is only applied to the policy inputs and not to
the value network inputs as the value function is not used during the deployment on the physical system.

%We add to the simulator markers (one for each fingertip and $3$ on the hand base) which correspond to the motion capture system used on the physical robot and slightly randomize their positions. The simulated markers are then used to compute the current positions of fingertips and the object.Following table summarizes these randomizations:

% bob: The quaternions do not have error added as Gaussian noise - instead, we choose a random axis and apply a small rotation around it.
\begin{table}
    \footnotesize
    \centering
    \caption{Standard deviation of observation noise.}
    
    \begin{tabular}{@{}lll@{}}
        \toprule
        \textbf{Measurement} & \textbf{Correlated noise} & \textbf{Uncorrelated noise} \\ \midrule
        fingertips positions & $1$mm & $2$mm \\
        object position & $5$mm & $1$mm \\
        object orientation & $0.1$rad & $0.1$rad \\ \hline
        fingertip marker positions & $3$mm & \\
        hand base marker position & $1$mm & \\
        \bottomrule
    \end{tabular}
\label{table:obs-noise}
\end{table}

\begin{table}
    \footnotesize
    \centering
    \caption{Standard deviation of action noise.}
    
    \begin{tabular}{@{}ll@{}}
        \toprule
        \textbf{Noise type} & \textbf{Percentage of the action range} \\ \midrule
        uncorrelated additive & 5\% \\
        correlated additive & 1.5\% \\
        uncorrelated multiplicative & 1.5\% \\
        \bottomrule
    \end{tabular}
\label{table:action-noise}
\end{table}

\paragraph{PhaseSpace tracking errors.}
Noise aside, readings of the motion capture markers from the PhaseSpace system might be occasionally unavailable for a short period of time due to instability of the service. To model such error in the simulator, we mask the fingertip markers with a small probability (0.2 per second) for 1 second so that the policy has a chance to learn how to interact with the environment while the system temporarily loses track of some markers. 

Furthermore, the markers might be occluded while in motion, causing a brief delay of readings of some fingertip positions. In the simulator, a small weightless cuboid site\footnote{A site represents a location of interest relative to the body frame in MuJoCo. Also see \url{http://mujoco.org/book/modeling.html\#site}.} is attached to the back of each nail and we consider a marker occluded whenever a collision with the site is detected as another finger or object is getting too close. If a fingertip marker is deemed occluded, we use its last available position readings instead of the current one.

\paragraph{Action noise and delay.}
We add correlated and uncorrelated Gaussian noise to all actions to account for an imperfect actuation 
system.
The detailed noise levels can be found in~\autoref{table:action-noise}.
%$0.03$ of additive correlated noise, $0.1$ of additive uncorrelated noise, and $0.03$ of multiplicative noise.
%
Moreover, the real system contains many potential sources of delays between the time that observations are sensed and actions are executed,
from network delay to the computation time of the neural network.
Therefore, we introduce a simple model of action delay to the simulator.
At the beginning of every episode we sample for every actuator whether
it is going to be delayed (with probability $0.5$) or not.
The actions corresponding to delayed actuator are delayed by one environment step, i.e. approximately $80$ms.
%All action coordinates are re-scaled to the range $[-1,1]$.

\paragraph{Timing randomization.}
We also randomize the timing of environment steps.
Every environment step is simulated as $10$ MuJoCo physics simulator steps
with $\Delta t=8\mbox{ms}+\mbox{Exp}(\lambda)$, where 
$\mbox{Exp}(\lambda)$ denotes the exponential distribution
and the coefficient $\lambda$ is once per episode sampled uniformly from the
range $[1250,10000]$.

\paragraph{Backlash model.}
The physical Shadow Dexterous Hand is tendon-actuated which causes a substantial
amount of backlash, while the MuJoCo model assumes direct actuation on the joints.
In order to account for it, we introduce a simple model of backlash which modifies
actions before they are sent to MuJoCo.
In particular, for every joint we have two parameters which
specify the amount of backlash in each direction, and are denoted $\delta_{-1}$ and $\delta_{+1}$,
as well as a time varying variable $s$ denoting the current state of slack.
We obtained the values of $\delta_{-1}, \delta_{+1}$ through
calibration.
%The values of in the range $1.25 \le \delta_{-1}, \delta_{+1} \le 4.25$, which means
%that it takes between $1/1.25\text{s}=800\text{ms}$ and $1/4.25\text{s}=235\text{ms}$
%to apply a full action.
At the beginning of every episode we sample the values of $\delta_{-1}, \delta_{+1}$
from the Gaussian distribution centered around the calibrated values with the standard deviation of $0.1$.
Let $a_{\text{in}} \in [-1,\,1]$ be an action specified by the policy.
%To simplify the exposition we assume that $a_{\text{in}}>0$.
Our backlash model works as follows: we compute the new value of the slack variable
$s'=[s+a_{\text{in}} \delta_{\textbf{sgn}(a_\text{in})} \Delta t]_{-1}^{+1}$,
compute the scaling factor
$\alpha=1-\left[\frac{|\textbf{sgn}(a_\text{in})-s|}{|s'-s|+\epsilon}\right]_0^1$,
where $\epsilon=10^{-12}$ is a constant used for numerical stability,
and finally multiply the action by $\alpha$:
$a_{\text{out}} = \alpha a_{\text{in}}$.
    
\paragraph{Random forces on the object.}
To represent unmodeled dynamics, we sometimes apply random forces on the object.
The probability $p$ that a random force is applied is sampled at the beginning of the episode from the loguniform distribution between $0.1\%$ and $10\%$.
Then, at every timestep, with probability $p$ we apply a random force
from the $3$-dimensional Gaussian distribution with the standard deviation equal to $1~m/s^2$ times the mass of the object on each coordinate and decay the force with the coefficient of $0.99$ per $80$ms.

%% lilian: we are not using the cube freezing wrapper.
% We also occasionally freeze the object itself in place and only unlock it whenever the policy performs a sequence of distinctively different actions. This is necessary because objects get easily stuck on the real system due to unmodeled non-convextities of the hand’s geometry.

\paragraph{Randomized vision appearance.} 
%
%For training the vision to state model, we use Unity to render images and employ domain randomization to obtain robust results.
We randomize the visual appearance of the robot and object, as well as lighting and camera characteristics.
The materials and textures are randomized for every visible object in the scene.
We randomize the hue, saturation, and value for the object faces around calibrated values from real-world measurements.
The color of the robot is uniformly randomized. Material properties such as glossiness and shininess are randomized as well. Camera position and orientation are slightly randomized around values calibrated to real-world locations.
Lights are randomized individually, and intensities are scaled based on a randomly drawn total intensity. After rendering the scene to images from the three separate cameras, additional augmentation is applied.
The images are linearly normalized to have zero mean and unit variance.
Then the image contrast is randomized, and finally per-pixel Gaussian noise is added. Details are in~\autoref{table:vision-randomization}.

\begin{savenotes}
\begin{table}
    \footnotesize
    \centering
    \caption{Vision randomizations.}
    
    \begin{tabular}{@{}ll@{}}
        \toprule
        \textbf{Randomization type} & \textbf{Range} \\ \midrule
        number of cameras & 3 \\
        camera position & $\pm$ 1.5 mm \\
        camera rotation & 0--3$^{\circ}$ around a random axis \\
        camera field of view & $\pm$ 1$^{\circ}$ \\
        \hline
        robot material colors & RGB \\
        robot material metallic level & 5\%--25\%\footnote{In units used by Unity. See \url{https://unity3d.com/learn/tutorials/s/graphics}.} \\
        robot material glossiness level & 0\%--100\%\footnotemark[\value{footnote}] \\
        \hline
        object material hue & calibrated hue $\pm$ 1\% \\
        object material saturation & calibrated saturation $\pm$ 15\% \\
        object material value & calibrated value $\pm$ 15\% \\
        object metallic level & 5\%--15\%\footnotemark[\value{footnote}] \\
        object glossiness level & 5\%--15\%\footnotemark[\value{footnote}] \\
        \hline
        number of lights & 4--6 \\
        light position & uniform over upper half-sphere \\
        light relative intensity & 1--5 \\
        total light intensity & 0--15\footnotemark[\value{footnote}] \\
        \hline
        image contrast adjustment & 50\%--150\% \\
        additive per-pixel Gaussian noise & $\pm$ 10\% \\
        \bottomrule
    \end{tabular}
\label{table:vision-randomization}
\end{table}
\end{savenotes}
