# Supplementary material for: ORRB -- OpenAI Remote Rendering Backend
Source: arXiv:1906.11633 source file (2019-06-26)
Supplement: Supplementary file 8 [file sim-full.tex]

\section{Simulated Environment}
\subsection{Deterministic Environment} \label{app:sim}

% We train our system in a simulated environment built within the MuJuCo physics engine~\citep{MuJoCo}.
% It consists of the 3D models of the Shadow Dexterous Hand
% and an object placed on the palm.
% The task is to manipulate the object into a desired goal orientation \num{50} times in a row, without dropping it.
% We start with a random initial object orientation and
% sample a new goal whenever the policy achieves the current one
% (within a tolerance of \SI{0.4}{\radian}).\footnote{I.e. we consider a goal as achieved if there exists a
% rotation of the object around an arbitrary axis with an angle smaller than \SI{0.4}{\radian}
% which transforms the current orientation into the desired one.}
% The model used for the hand is similar to the one used in the OpenAI~Gym robotics environments
% \citep{plappert2018multi} but has been improved to match the physical hand 
% (full description in Appendix~\ref{app:model-calibration}).

% The hand has \num{24} degrees of freedom (DoFs), \num{16} of which 
% can be controlled independently.  The remaining \num{8} joints (which are the joints between the finger proximal, middle and distal segments)
% are coupled.
% In contrast to the actual mechanical tendon-based design of the hand,
% we use a simplified simulated actuation model that applies torques directly to the joints.

\paragraph{Simulation.} Our environment is based on the OpenAI Gym robotics environments described in~\citep{plappert2018multi}. We use MuJoCo for simulation~\citep{MuJoCo}.

\paragraph{States.}
The state of the system is \num{60}-dimensional and consists of angles and velocities of all robot joints as well as the position, rotation and velocities (linear and angular) of the object.
Initial states are sampled by placing the object on the palm in a random orientation
and applying random actions for $100$ steps (we discard the trial if the object is dropped in the meantime).

\paragraph{Goals.}
The goal is the desired orientation of the object represented as a quaternion.
A new goal is generated after the current one has been achieved within a tolerance of \SI{0.4}{\radian}.\footnote{I.e. we consider a goal as achieved if there exists a
rotation of the object around an arbitrary axis with an angle smaller than \SI{0.4}{\radian}
which transforms the current orientation into the desired one.}

\paragraph{Observations.}
Described in \autoref{table:policy-inputs}.
%The policy is given the fingertips and the object positions ($18D$), as well as the %difference between the desired
%orientation of the object and the current one represented as a quaternion ($4D$).
%It is trivial to track the fingertip positions and object pose in the simulator, which are used as the input for the policy network. 
%We are able to easily gather several additional measurements in the simulator that cannot be tracked in the physical system, such as hand joint angles and velocities and feed into the value network to facilitate the training. Joint angles or velocities are not needed from the physical system, as the value network is not used when deploying policy on the robot.

\paragraph{Rewards.} \label{sec:reward}
The reward given at timestep $t$ is $r_t=d_t-d_{t+1}$, where
$d_t$ and $d_{t+1}$ are the rotation angles between the desired 
and current object orientations before and after the transition, respectively.
We give an additional reward of $5$ whenever a goal is achieved with the tolerance of \SI{0.4}{\radian}
(i.e. $d_{t+1}<0.4$) and a reward of $-20$ (penalty) whenever the object is dropped.

\paragraph{Actions.}
Actions are \num{20}-dimensional and correspond to the desired angles of the hand joints.
We discretize each action coordinate into $11$ bins of equal size.
Due to the inaccuracy of joint angle sensors
on the physical hand (see Appendix~\ref{app:hardware}), actions are specified
relative to the current hand state.
In particular, the torque applied to the given joint in simulation is equal to $P*(s_t+a-s_{t'})$, where
$s_{t}$ is the joint angle at the time when the action was specified,
$a$ is the corresponding action coordinate, 
$s_{t'}$ is the current joint angle,
 and $P$ is the proportionality coefficient.
For the coupled joints, the desired and actual positions represent the sum of the two joint angles.
All actions are rescaled to the range $[-1,1]$.
To avoid abrupt changes to the action signal, which could harm a physical robot,
we smooth the actions using an exponential moving average\footnote{We use a coefficient of $0.3$ per 80ms.}
before applying them (both in simulation and during deployments on the physical robot).

\paragraph{Timing.}
Each environment step corresponds to \SI{80}{\ms} of real time and consists of \num{10} consecutive MuJoCo steps, each corresponding to \SI{8}{\ms}.
The episode ends when either the policy achieves \num{50} consecutive goals, the policy fails
to achieve the current goal within \num{8} seconds of simulated time, or the object is dropped.
