# Supplementary material for: ORRB -- OpenAI Remote Rendering Backend
Source: arXiv:1906.11633 source file (2019-06-26)
Supplement: Supplementary file 9 [file vision.tex]

% \subsection{Vision Model Details}
% \label{app:vision_model_details}

% We use a vision-to-state deep convolutional neural network to estimate the location and orientation of the manipulated object. 
% The architecture of the network is described in \autoref{sec:vision_model_arch}.

% \todo{Alex: move to a table with hyperparameters in App. F}

% We use a vision-to-state deep convolutional neural network to estimate the location and orientation of the block or octagonal prism. 
% The architecture of the network is described in Section~\label{sec:vision_model_arch}.
% We trained our models using the Adam optimizer with a learning rate of $0.0005$ that was decayed by a factor of $2$ every $20000$ batches. 
% We used batches of size $64$ consisting of $32$ images synthetic images. 
% We trained for $400000$ batches and regularized the network with a weight decay of $0.001$. 
% Images were downsized to $200 \times 200$ throughout. 
